# Supplementary material for: Warping of Radar Data into Camera Image for Cross-Modal Supervision in Automotive Applications
Source: arXiv:2012.12809 source file (2022-06-20)
Supplement: Supplementary file 1 [file appendix.tex]

%\newpage

\appendices

\newlength\figH
\newlength\figW

\section{Further evaluation of DRISFwR}\label{sec: drisfwrAppend}
\label{se:drisfwrEvalExtension}
To support the scene flow evaluation from the main text of this paper, we provide qualitative comparison of the three compared scene flow algorithms in Fig. \ref{fig:drisfwrEval}.

\begin{figure}[h]%[H]
\centering
    \scalebox{0.9}{\input{DRISwR/Eval/evaluation.tex}}
    \caption{\textbf{Qualitative results of scene flow algorithms on test data examples}: From top-to-bottom: radar FoV coverage within RGB image, scene flow error of $\text{HD}^3$, scene flow error of DRISF, scene flow error of DRISFwR. Our method was able to achieve lower object scene flow errors in general. Notice, that only foreground objects in radar FoV are taken into account for evaluation, thus remaining pixels are colored black.}
    \label{fig:drisfwrEval}
\end{figure}

It can be seen, that in all examples DRISFwR provides better results than DRISF and especially as the scene flow algorithms without strong motion priors.

To investigate the effect of high dynamic ego-motion to scene flow accuracy, the scene flow error between the reference scene flow and the scene flow estimations based on DRISF and DRISFwR are plotted in Fig. \ref{fig:drisfwrEval2} against the ego-vehicle's rotational motion (yaw rate). It can be seen, that the scene flow errors are nearly constant. We conclude, that scene flow estimates by DRISF and DRISFwR are capable of handling high dynamic ego-motion trajectories.

%
%\begin{figure}[h]
%%\begin{center}%
%
%\subfigure[MAE]{
%    %\scalebox{.7}{\hspace{-2cm}\input{Auswertung\DRISF.tex}}
%    \begingroup
%    \inputencoding{latin1}
%    \input{S:/GE-E/E-ED/E-ED-DAS/E-ED-DAS-SW/E-ED-DAS-SW4/01_Mitarbeiter/Grimm/save/LIPPI_Dataset/05_11_2019/evaluation/sceneflow_evaluation/sceneFlow_DGPSCameraGT/2/sceneflowEvaluation1.tex}
%    %\scalebox{.7}{\hspace{0.001cm}\input{Auswertung/sceneflowEvaluation.tex}}
%    \endgroup
%    }
%    \subfigure[error rate]{%[c]{0.5\textwidth}
%    %\scalebox{.7}{\hspace{-2cm}\input{Auswertung\DRISF.tex}}
%    \begingroup
%    \inputencoding{latin1}
%    \input{S:/GE-E/E-ED/E-ED-DAS/E-ED-DAS-SW/E-ED-DAS-SW4/01_Mitarbeiter/Grimm/save/LIPPI_Dataset/05_11_2019/evaluation/sceneflow_evaluation/sceneFlow_DGPSCameraGT/2/sceneflowEvaluation2.tex}
%    %\scalebox{.7}{\hspace{0.001cm}\input{Auswertung/sceneflowEvaluation_error.tex}}
%    \endgroup
%    }
%    
%  
%    %\end{center}
%
%    \caption{\textbf{Motion analysis}. Cumulative distribution function of scene flow error versus yaw-rate. On average DRISFwR reduces scene flow deviation and error rate even when ego-vehicle is cornering}
%    
%    \label{fig:drisfEvaluation}
%\end{figure}

%
\begin{figure}[H]%[tbh]
\centering
\input{sceneflow_evaluation/sceneFlow_DGPSCameraGT/2/sceneflowEvaluation1.tex}
     \caption{\textbf{Motion analysis}. Cumulative distribution function of scene flow error versus yaw-rate. On average DRISFwR reduces scene flow deviation even when ego-vehicle is cornering.}
    \label{fig:drisfwrEval2}
\end{figure}

\section{Automatic warping error handling via loss scale-space}\label{ss: scalespaceLoss}
Even though the DRISFwR approach is able to align the estimated scene flow with respect to the radar's RD spectrum, warping from the radar spectrum to camera image can be incorrect if there is a remaining error in $v_r(\boldsymbol{\xi})$ and $|\textbf{x}_r|$, which exceeds the resolution of the radar. 
%As a consequence, it leads to performance degradation in \gls{CNN} training. 
We borrow the concept of scale space from, which is used in optical flow estimation for decades, see e.g. \cite{Yang99}, to mitigate this effect, we create image pyramids by subsampling the NN's prediction and, thus, virtually reduce the radar's RD resolution depending on scale-level $s$. Here $3$ scale-levels are used.

Subsampling is performed via 2D-average pooling on prediction $a$ in RD grid, weighted by RD bin power
\begin{equation}
\phi_\text{pred., scaled} \Big( \phi_\text{pred.}(\textbf{p}), \mathcal{RD(\textbf{p})}, s\Big) = \frac{\sum_{ \textbf{p}_v \in \mathcal{V}(s) }  \mathcal{RD}(\textbf{p}_v) \phi_\text{pred.}(\textbf{p}_v)   }{ \sum_{ \textbf{p}_v \in \mathcal{V}(s) }   \mathcal{RD}(\textbf{p}_v)  },
\end{equation}
where $\mathcal{V}(s)$ is the spatial region around the pixel $\textbf{p}$. A theoretical analysis of average pooling can be found in \cite{Boureau10}.

\subsection{Toy example}

The outcome of the scalespace prediction is depicted in\mbox{ Fig. \ref{fig:scaleSpaceLoss_example_0}} for a toy example. A region of a real recorded $\mathcal{RD}$ map is shown on the left. On the right hand side, synthetic angle predictions are shown, whereas the ground truth angle was $0^\circ$ and all DoA predictions below a certain SNR threshold in $\mathcal{RD}$ were filled with random angle estimates. We select one pixel in the $\mathcal{RD}$ which is adjacent to local maxima and therefore simulates the erroneous velocity estimate by the reference sensor system. The angle estimates for this pixel at scale-levels of $s=0$ and $s=2$ are given in the image. We can see, that $s=2$ provides an estimate closer to the ground truth angle of $0^\circ$ and therefore less aspiration to be modified by the optimizer during \gls{NN} training. 
\setlength{\figW}{\columnwidth}
\setlength{\figH}{0.7\figW}

\begin{figure}[H]
\centering
\input{ScaleSpaceLoss/LossDescription/tikzOutput_1.tex}
\caption{\textbf{Toy example of scale space prediction:} Die Übersicht der Schichten.}
\label{fig:scaleSpaceLoss_example_0}
\end{figure}

Hereafter, the prediction on every scale space level is warped into the camera image and compared to the corresponding camera label to create a per scale loss, whose sum gives the overall training objective, see Fig. \ref{fig:scaleSpaceLoss}. The effective RD resolution is bisected at each scale-level.

\begin{figure}[H]
\centering
    \scalebox{0.75}{\hspace{-2cm}\input{ScaleSpaceLoss/image.tex}}
    \caption{\textbf{Loss in scale-space:} As accurate warping operations require an accuracy better than the RD resolution, we downscale RD grid to virtually reduce the resolution. This helps mitigate warping errors to forestall the training process. }     
\label{fig:scaleSpaceLoss}
\end{figure}

\subsection{Cost function}

\begin{equation}
l_{\phi-\text{Net}} = \sum_{\textbf{p} \in \mathcal{P}_\text{train} }
\sum_{s \leq S }
\frac{1}{s} \big|\phi_\text{reference}\left(\textbf{p}\right) - \phi_\text{predict, cam}\left(\textbf{p}, s\right)\big|, 
\end{equation}

\subsection{Evaluation}

To test the influence of the scale-space loss, we designed an ensemble of NNs with the following configuration. 

\begin{table}[h]
\centering
\caption{\textbf{NN architectures and their configurations}.}
\label{tab:nnArchitectures}
\begin{tabular*}{0.45\textwidth}{lccc}
\toprule
Name & kernel size & layer modifier (t) & loss scales \\
\midrule
$\text{NN}_0$ & $1\times1$ & 3 & 1\\
$\text{NN}_1$ & $1\times1$ & 3 & 3\\ 
$\text{NN}_2$ & $3\times3$ & 1 & 1\\
$\text{NN}_3$ & $3\times3$ & 1 & 3\\
\bottomrule
\end{tabular*}
\end{table}

The performance of different DoA estimators in terms of \gls{MAE} is shown in Fig. \ref{fig:qualityCurveDoA} for the azimuth interval of $[-30^\circ, 30^\circ]$. In addition to \gls{NN}-based estimators we include the performance of a phase-monopulse (PM) \cite{Stabilito61} DoA estimator and Bartlett beamforming (BF) \cite{Krim96} as baseline algorithms which do not require a training phase. It can be seen, that the (3x3) NN estimator achieves the lowest \gls{MAE} over the entire SNR range. It is also superior the the (1x1) NN architectures. This suggests, that neighboring RD-map pixels carry valuable information that can be used for a better DoA estimation. A possible explanation for this is (a) the windowing performed before computing the FFT based RD grid, which smears energy over multiple pixels, and (b) that geometrically neighboring pixels in the camera image tend to occupy neighboring locations in the RD-grid. Furthermore, we can see that the NN with introduced scale level loss performed equal ($\text{NN}_2$ vs. $\text{NN}_3$) or worse ($\text{NN}_0$ vs. $\text{NN}_1$) that the NN without scale space loss. This suggests, that the selected scale space loss is detrimental for DoA training. 

%\newlength\figH
%\newlength\figW
\setlength{\figH}{10cm}
\setlength{\figW}{\columnwidth }
\begin{figure}[ht]
\begingroup
 \inputencoding{latin1}  \input{Results/Azimuth/Azimuth_ROC_curve_usedInPaper_new.tex}
\endgroup
\caption{\textbf{Performance of DoA estimation methods:} 
Mean Absolute Error of azimuth estimation of different DoA estimators and performance of moving target indication (MTI).}
\label{fig:qualityCurveDoA}
\end{figure}

Even though, the overall MAE was worse for the NNs using scale-space loss, we can see minor benefit in 
$\text{NN}_0$ vs. $\text{NN}_1$, where the high MAE region at around $-45^\circ$ was removed. Similarly, but more faint is the result for $\text{NN}_2$ vs. $\text{NN}_3$. However, in other azimuth regions, e.g. $45^\circ$ we can spot larger MAE values when using the scale space loss.

\setlength{\figH}{7cm}
\setlength{\figW}{0.75\columnwidth }
\begin{figure}[h]
\centering     %%% not \center
\subfigure[$\text{NN}_0$]{\label{fig:a}  \input{Results/Azimuth/SnrVsAzimuth/newRoutine_3_algo_0_azLimit_30_MAE.tex}}
\subfigure[$\text{NN}_1$]{\label{fig:a}  \input{Results/Azimuth/SnrVsAzimuth/newRoutine_3_algo_1_azLimit_30_MAE.tex}}
\subfigure[$\text{NN}_2$]{\label{fig:b} \input{Results/Azimuth/SnrVsAzimuth/newRoutine_3_algo_2_azLimit_30_MAE.tex}}
\subfigure[$\text{NN}_3$]{\label{fig:b} \input{Results/Azimuth/SnrVsAzimuth/newRoutine_3_algo_3_azLimit_30_MAE.tex}}
\subfigure[PM]{\label{fig:b} \input{Results/Azimuth/SnrVsAzimuth/newRoutine_3_algo_4_azLimit_30_MAE.tex}}
\subfigure[BF]{\label{fig:b} \input{Results/Azimuth/SnrVsAzimuth/newRoutine_3_algo_5_azLimit_30_MAE.tex}}
\caption{\textbf{MAE in dependency on azimuth and SNR:} Mean Absolute Error of different DoA estimators.}
\label{fig:qualityCurveDoA_hist}
\end{figure}

\section{Target detection via neural network}\label{ap:targetDetection}\label{sec: targetDetectionAppend}

As another classical radar signal processing application, beside DoA estimation, target detection can be performed via NN. Compared to DoA, we found that automatic label generation is significantly more challenging for target detection. For the DoA application, the cameras provides direct resolution in the label units and thus the labels can be seen as ground truth. However, for target detection the the reference labels must be estimated as the reference system has no innate understanding of what the radar sensor sees and what not. %\inred{Our label estimation approach for target detection is arguable, but we still wanted to share our current research to others and therefore we decided to include this section into appendix rather than the main section of this paper.  Mit dieser Aussage diskreditierst Du die ganze Untersuchung!! Also wuerde ich sie weglassen!}

\subsection{Label generation}
%Classical target detection typically performs hypothesis tests on the received signal power and compares it to a noise level estimate. Once the receive power exceeds the noise level estimate significantly, a real target is assumed to be responsible for the signal. 
%Here, we follow our results from Sec. \ref{se:rcsResults}, which concludes that signal power is proportional to the aspect angle between radar and any surface normal to provide reference labels for neural network based target detection on radar spectrum. 

%\textcolor{red}{Label threshold beschreiben}
%

The neural network (called $\text{TD}-\text{Net}$ in the following) is trained against virtual reflectors $\Omega_\text{GT}$ from reference system, which are deduced based on geometric properties of the reflecting objects in the dense depth map. From literature, e.g. \cite{Mes06, Yang06}, it is well known, that radar reflectivity highly depends on the aspect angle between radar on reflector surface. We calculate the aspect angle with the cosine similarity via scalar projection as follows,
\begin{equation}
\cos\left( \angle \left( \textbf{x}_R, \textbf{n}_R \right) \right) = \frac{\textbf{x}_R \cdot \textbf{n}_R}{\| \textbf{x}_R\| \| \textbf{n}_R\|},
\label{eq: aspectAngle}
\end{equation}
where $\textbf{x}_R$ is the ray direction and $\textbf{n}_R$ is the surface normal from dense depth seen from radar perspective. Surface normal is calculated from $\textbf{x}_R$, by taking cross product of quadrilaterals in image plane. The entity of cosine similarity for all pixels is consolidated in $\mathcal{A}$.

%Examples of aspect angle are visualized in Fig. \ref{fig:targetDetection}, left column.

As the $\text{TD}-\text{Net}$ training requires one-hot encoded labels, we seed virtual target label in camera image, when the cosine similarity value exceeds 
\begin{equation}
|\cos\left( \angle \left( \textbf{x}_R, \textbf{n}_R \right) \right)| \geq 0.5.
\label{eq: aspectAngle2}
\end{equation}
 This value is inspired by Rayleigh criterion \cite{Woodhouse06} describing surface smoothness related to wavelength and by empirical investigation. Further physical modeling of reflectivity based on electromagnetic properties is not carried out and postponed for future investigations.

\subsection{Network architecture}
$\text{TD}-\text{Net}$ has similar architecture as $\phi-\text{Net}$, except for last layer being single output with sigmoid activation to model per-pixel confidence $\Omega$ of significant reflection. Input data for the network is the RD-map from radar spectra. 

\subsection{Optimization}
For network optimization binary cross entropy is utilized as cost function,
\begin{equation}
  l_{\text{TD}-\text{Net}} = - \sum_{\substack{\mathcal{P}_\text{radar} }} \sum_{s \leq S }
\frac{1}{s}
\Big(\Omega_\text{GT}\log(\Omega) + (1-\Omega_\text{GT})\log(1-\Omega)\Big).
\end{equation}

\subsection{Results}
Qualitative results are visualized in Fig. \ref{fig:targetDetection2} for the reference labels, the neural network predictions and a classical CFAR estimation as reference. 

It can be seen, that the color distribution between the reference mask and the predicted mask in camera image mostly match. One major difference between the NN based prediction and the CFAR prediction is that the NN is that the later one does only categorical prediction (either target or no-target). Apart from that, we found, that the NN based predictions for target detection produces similar results as the CFAR target detection algorithm.

%we did not find a major difference between NN based target detection and CFAR based target detection.  %\inred{also warum das dann ueberhaupt bringen?}

As declared, the reference labels for target detection highly depend on the utilized vision model (see eq. \ref{eq: aspectAngle2}) and therefore we disclaim to provide quantitative results. 

%\begin{figure*}[tb]
%\centering
%    \scalebox{1}{\input{Results/TargetDetection/Supplement/evaluation_supplement.tex}}
%    \caption{\textbf{Qualitative results of target detection on test data examples}. %From left-to-right: reference targets (brightness is aspect angle), target detections (via our method and CFAR) warped onto camera image (brightness is predicted target probability) and target detections (via our method and CFAR) in radar spectra (brightness is predicted target probability). Only pixels in radar FoV are visualized and color scales with target probability. During training, the network is adjusted so that ``prediction (warped)'' equals ``reference''.
%From left-to-right: RGB image with color coded target labels, RGB image with color coded target predictions from NN, RGB image with color coded target predictions from CFAR, RD-map with color coded target prediction from NN, RD-map with color coded target prediction from CFAR  .}
%    \label{fig:targetDetection2}
%\end{figure*}

\begin{figure*}[tb]
\centering
    \scalebox{1}{\input{Results/TargetDetection/Supplement/evaluation_supplement2.tex}}
    \caption{\textbf{Qualitative results of target detection on test data examples}. %From left-to-right: reference targets (brightness is aspect angle), target detections (via our method and CFAR) warped onto camera image (brightness is predicted target probability) and target detections (via our method and CFAR) in radar spectra (brightness is predicted target probability). Only pixels in radar FoV are visualized and color scales with target probability. During training, the network is adjusted so that ``prediction (warped)'' equals ``reference''.
From left-to-right: RGB image with color coded target labels, RGB image with color coded target predictions from NN, RGB image with color coded target predictions from CFAR, RD-map with color coded target prediction from NN, RD-map with color coded target prediction from CFAR, RD-map.}
    \label{fig:targetDetection2}
\end{figure*}

%\begin{figure*}[tb]
%\centering
%    \scalebox{1}{\input{Results/Class/Supplement/evaluation_supplement.tex}}
%    \caption{\textbf{Qualitative results of target detection  on test data}. From left-to-right: reference targets (brightness is aspect angle), target detections (via our method and CFAR) warped onto camera image (brightness is predicted target probability) and target detections (via our method and CFAR) in radar spectra (brightness is predicted target probability). Only pixels in radar FoV are visualized and color scales with target probability. During training, the network is adjusted so that ``prediction (warped)'' equals ``reference''.}
%    \label{fig:targetDetection2}
%\end{figure*}

\section{Semantic segmentation via neural network}\label{sec: semanticSegmentationAppend}
\label{ap:semanticSegmentation}
Another application for our proposed pipeline is the semantic segmentation of RD spectrum data. Each pixel in RD grid is classified as being stationary (against the world), moving pedestrian, moving vehicle or background. %Motivated by the recent success of two-stage classifier networks \cite{Girshick14,He18, Lin18}, semantic segmentation  task is split into two subtask (1) target detection, which identifies significant reflectors in the spectra and (2) classification, which assigns class probability for the pixels.

In \cite{Grimm17a, Grimm17b} we proposed a hypothesis test for the detection of moving radar targets based on their relative radial velocity and DoA measured by a radar. 

%This hypothesis test was simple, yet very accurate, thus we decide to inherit it into the classification network. The modified version of the hypothesis test is given as:
%\begin{equation*}
%p(p == c_\text{moving}) = \text{sig}\big( \rho\left(\mu_E\right) - \sigma_e \cdot Q^{-1}\left( \alpha/2\right) \big)
%\end{equation*}
%were 
%\begin{equation*}
%\text{sig}\left(t\right) = \frac{1}{1-e^{-t}}
%\end{equation*}
%being the Sigmoid function and 
%\begin{equation*}
%\rho\left(t\right) = \sqrt{t^2 + 10^{-10}}
%\end{equation*}
%being the Charbonnier penalty. Sigmoid (``soft-step'') was applied as the differentiable approximation of the step function. Charbonnier penalty was used as the differentiable alternative of the $\| t\|$ to cover prefix of the error ($\mu_E$). $\mu_E$ and $\sigma_e$ are the difference in between measured radial relative velocity and expected velocity for stationary targets and expected velocity variance. $Q^{-1}(\alpha/2)$ is the inverted (Gaussian) tail distribution function under the level of significance $\alpha$. With this, instead of being categorical $p(p == c_\text{moving})$ now converts into a continuous variable $\in [0,1]$, which increases for moving targets/objects and decreases for stationary objects. The value is computed on pixel level in the RD-map and is illustrated for one example in Fig. \ref{fig:movingType}.

This hypothesis test is simple, yet very accurate, thus we decide to inherit it into the classification network in modified form. The modified and differentiable version of the hypothesis test is given as
\begin{equation}
\text{Pr}(p == c_\text{moving}) = \exp\bigg\{ \frac{\mu_E^2}{\left( \sigma_E \cdot  Q^{-1}\left( \alpha/2\right)\right)^2}  \bigg\},
\label{eq:HypothesisTest}
\end{equation}
were $\mu_E$ and $\sigma_e$ are the difference  between measured radial relative velocity and expected velocity for stationary targets and expected velocity variance. $Q^{-1}(\alpha/2)$ is the inverted (Gaussian) tail distribution function  under the level of significance $\alpha$. Gaussian activation function was used, motivated by the modeling of $\mu_E$ as being Gaussian distributed (and producing sharper decisions compared to Softstep-function). With this, instead of being categorical $\text{Pr}(p == c_\text{moving})$ now converts into a continuous variable $\in [0,1]$, which increases for stationary targets/objects and decreases for moving objects. The value is computed on pixel level in the RD-map ($\mathcal{MT}$) and warped into camera image ($\mathcal{MT}_C$) with one scene example illustrated in Fig. \ref{fig:movingType}.

\begin{figure}[h]
\centering
    \scalebox{1.}{\input{TeacherStudentArchitecture/movingType.tex}}
    \caption{\textbf{Example of moving type indication}. Top-row: RGB image, RD-map; Bottom-row: Moving target confidence (brighter values mean higher confidence) estimated by neural network in camera image and in RD-map. The ego-vehicle was moving with the postal truck following.}
    \label{fig:movingType}
\end{figure}

\subsection{Network architecture}
%The neural network architecture ($\Psi$-Net) is similar to the architecture of $\text{TD}-\text{Net}$, but the the number of input channels is increased to incorporate the results of the hypothesis test. The output channel size is also increased to 3 to provide multi-label confidence per class. 

The NN architecture ($\Psi$-Net) is similar to $\phi$-NN, except that at first layer, the 3D radar spectra and the output of stationary target detection step are convolved individually and the outcome is concatenate towards the second layer. The output channel size is also increased to 3 to provide multi-label confidence.

%The subsequent semantic segmentation is performed via regular CNN architecture and hence its classification task, the network is named $\Psi$-Net subsequently. The network operates as multi-label classification and thus allows multiple labels per RD-map pixel.  

\subsection{Optimization}
For training of $\Psi$-Net, focal-loss \cite{Lin17} was evaluated between semantic segmentation prediction on RD-map projected into camera image $\Psi$ and the semantic segmentation from teacher network $\Psi_\text{GT}$ native in camera image. The class predictions of $\Psi$-Net are \{``stationary'', ``pedestrian'', ``vehicle'', ``background'' \} which express  if a RD-map pixel stationary or a moving pedestrian or vehicle. The focal-loss cost function  is utilized with cost scaling $w_c = [1, 500, 10]$ to mitigate class-imbalance and empirically found to achieve better classification,

%We model the semantic segmentation task as multi-class classification problem via softmax activation and multinomial cross entropy with focal-loss, and thus enforce class activations $a_i$ to be mutual exclusive
%\begin{equation}
%a_i = \frac{\exp{c_i}}{\sum_j\exp{c_j}}.
%\end{equation}
%Due to class imbalance, we found it helpful to utilize focal-loss
%Since the label frequency for negative examples on average is higher than positives, we apply class balancing and reciprocally scale positive examples in the cross-entropy loss function as $w_c = [1, 500, 10]$ which was the class frequency of a typical example image.
%The focal-loss cost function \cite{Lin18} is utilized with cost scaling $w_c = [1, 500, 10]$ to mitigate class-imbalance and empirically achieve better classification.
%
%
%\begin{equation}
%l_{C-\text{NN}} = 
%- 
%\sum_{\substack{p \in \text{FoV}_\text{RADAR} \\ p \in \Omega \geq 0.5 \\ Class==i }}
%w_c (1-a_i)^{2} \log\left( a_i\right).
%\end{equation}
%Notice that only pixels are involved into the cost function, where target detection network proposes activation $\Omega$ larger than 0.5 to focus on target proposals only.

%The focal-loss cost function \cite{Lin17} is utilized with cost scaling $w_c = [1, 500, 10]$ to mitigate class-imbalance and empirically found to achieve better classification,

%\begin{equation}
%l_{C-\text{NN}} = 
%- 
%\sum_{\substack{p \in \text{FoV}_\text{RADAR} \\ p \in \Omega \geq 0.5 \\ Class==i }}
%w_c (1-a_i)^{2} \log\left( a_i\right).
%\end{equation}

\begin{equation}
\begin{split}
  l_{\Psi-\text{NN}} = - \sum_{\mathcal{P}_\text{radar}} \sum_{s \leq S }
  \frac{1}{s}
\Big(
w_c (1-\Psi)^{2} \Psi_\text{GT}\log(\Psi) + \\ \Psi^2(1-\Psi_\text{GT})\log(1-\Psi)\Big).
\end{split}
\end{equation}

Label for ``stationary'' is set high, if semantic segmentation classifies pixel as pedestrian or vehicle, its DRISFwR scene flow deviates from stationary scene flow only marginal in its radial component ($\SI{0.6}{\meter\per\second}$) and if $\Omega_\text{GT}$ is true. Remaining labels for ``pedestrian'' and ``vehicle'' come from semantic segmentation on RGB image.

\subsection{Results}
%\begin{figure}[tb]
%\centering
%    \scalebox{1}{\input{Results/Class/evaluation2.tex}}
%    \caption{\textbf{Qualitative results of class prediction on test data}. From left-to-right: reference targets (brightness is aspect angle), target detections projected into camera image (brightness is predicted target probability) and target detections in radar spectra (brightness is predicted target probability). Only pixels in radar FoV are visualized and color scales with target probability.}
%    \label{fig:classification}
%\end{figure}
%
%\begin{figure*}[tb]
%\centering
%    \scalebox{1}{\input{Results/Class/Supplement2/evaluation_supplement.tex}}
%    \caption{\textbf{Qualitative results of semsnatic segmentation  on test data}. From left-to-right: reference targets (brightness is aspect angle), target detections (via our method and CFAR) warped onto camera image (brightness is predicted target probability) and target detections (via our method and CFAR) in radar spectra (brightness is predicted target probability). Only pixels in radar FoV are visualized and color scales with target probability. During training, the network is adjusted so that ``prediction (warped)'' equals ``reference''.}
%    \label{fig:targetDetection2}
%\end{figure*}

Qualitative results are visualized in Fig. \ref{fig:semanticSegmentation}. It can be observed, that the color of the semantic mask predicted by the neural network and warped into camera image mostly resembles the reference label mask and that the predictions are reasonable. We found, that the main difference between the predicted semantic mask and the reference mask occurs in different distributions of intensity in the images. This can be explained, as the reference masks intensity is based on aspect angle, while the NN learned to create mask intensity based on SNR value in the RD-map. One example of this can be seen by comparing the reference labels and the predictions of the third example in Fig. \ref{fig:semanticSegmentation}. The reference labels of the parking car, shown left in the images, are significantly noisy whilst the predictions occur reasonable. The fact that the $\Psi$-Net was still able to estimate reasonable semantic masks in real world scenes suggests, that (a) utilizing aspect angle to estimate reference masks is appropriate and (b) the presented algorithms for robust NN training (scalespace costs and optimization criteria) in conjunction with large amounts of training data helped to train the NN despite significant label noise. Due to significant label noise, we disclaim to provide quantitative results.

\begin{figure}[tb]
\centering
    \scalebox{1}{\input{Results/Class/Supplement2/evaluation_supplement_singleColumn.tex}}
    \caption{\textbf{Qualitative results of semantic segmentation  on test data examples}. %From left-to-right: reference targets (brightness is aspect angle), target detections (via our method and CFAR) warped onto camera image (brightness is predicted target probability) and target detections (via our method and CFAR) in radar spectra (brightness is predicted target probability). Only pixels in radar FoV are visualized and color scales with target probability. During training, the network is adjusted so that ``prediction (warped)'' equals ``reference''.
    From left-to-right: RGB image with color coded semantic mask labels, RGB image with color coded semantic predictions from NN, RD-map with color coded semantic predictions.
    }
    \label{fig:semanticSegmentation}
\end{figure}

\section{Estimating Radar SNR from camera}\label{sec: snrEstimationnAppend}
\label{ap:rcsEstimation}
The main contribution of this paper was the design of a teacher-trainer framework for radar based NN training against labels from camera vision models. However, with minor modifications to the framework, see Fig. \ref{fig:ablaufdiagram10}, it is also possible to train camera fed estimators against radar data. 

\begin{figure}[h]
\centering
    \scalebox{0.75}{\hspace{-2cm}\input{Flowchart_nn_and_gt3_.tex}}
    \caption{\textbf{Overview of the model pipeline for camera based estimators:}  Utilization of the reference sensors (lidar \& camera) and the radar for the supervised training of a neural-network operating on camera data.}
    \label{fig:ablaufdiagram10}
\end{figure}

As an example of this approach we train a NN to estimate the radars RD-map SNR values from camera input. Therefore, we use the notation 
SNR-NN to decribe this specific network. We found this approach useful as it might be helpful for the development of e.g. radar raytracing software.

%Utilizing our proposed approach for training radar operating student neural networks, the radar can be used as a teacher to train a camera \& lidar based neural network (RCS-NN) as well. This allows us to learn power maps based on image feature maps provided from camera and lidar reference system. The basic approach can be seen in Fig. \ref{fig:ablaufdiagram4}. %Notice, that only the position of the neural network in the graph has changed.

\subsection{Network input feature maps}
As inputs for the SNR-NN, the dense depth map, semantic mask, aspect angle image and the camera RGB image are provided. The depth map is provided, as range is an important power modulation factor in radar range equation \cite{schroeder2013system}. Semantic mask is used, as by physic radar-cross-section (RCS) and thus SNR highly depends on material characteristics. The idea was, that once the NN knows class properties, it can generate a intrinsic guess of material properties used in different traffic participants. Aspect angle image was used, to provide the NN a prefabricated idea on how much emitted power from the radar is redirected back to the radar as reflection or transmissioned into space. Additionally the raw rgb image is provided, to allow the NN to extract visual cues itself, which are not covered by the pre-processed image features.

\subsection{Network architecture}
The DNN architecture is fully convolutional with ReLU activations on every layer. The convolutions are $3\times3$ with unit stride and following channel count $[16, 32, 64, 32, 16, 16, 1]$. The input feature maps are reprocessed  via single layer convolution separately, where each feature map results in 4 intermediate channels. Intermediate channels from feature maps are then concatenated as input for the neural network.

\subsection{Optimization}
Assuming Swerling type 3 fluctuations (see e.g. \cite{Mes06}) in the reflected radar echo, we can model the observed RCS $\sigma$ as a Chi-squared distribution from the true RCS $\overline{\sigma}$

\begin{equation}
p( \sigma | \overline{\sigma} ) = \frac{4\sigma}{\overline{\sigma}^2}e^{-2\frac{\sigma}{\overline{\sigma}}}.
\label{eq:swerling}
\end{equation}

Hence the received signal power linear scales with the RCS (see radar range equation), we obtain loss function for the neural network by calculation of the maximum-likelihood (ML) estimator for $\overline{\sigma}$
via derivative of log-likelihood functions 
\begin{equation}
\log\left( L\left(p\right) \right) = \log{ \left( 
\prod_i \frac{4\sigma}{\overline{\sigma}^2}
e^{-2\frac{\sigma_i}{\overline{\sigma}}} 
\right) }
\label{eq:ml1}
\end{equation}
as
\begin{equation}
\frac{\partial \log( L(p) ) }{\partial \overline{\sigma}} = \sum_i^N (\sigma_i - \overline{\sigma})
\label{eq:ml2}
\end{equation} 
and
\begin{equation}
\overline{\sigma}^{(ML)} = \frac{\sum \sigma_i}{N}.
\label{eq:ml3}
\end{equation}

From Eq. \ref{eq:ml2} we see, that in order to optimize SNR estimate, we need to minimize the difference between radar measured SNR $\mathcal{RD}_C$ (warped power spectra from radar) and estimated SNR $\mathcal{RD}_\text{prediction}$ (estimated power from \text{SNR}-\text{NN}). Which results in the utilized loss function as 
\begin{equation}
  l_{\text{SNR}-\text{NN}} = \sum_{\substack{\mathcal{P}_\text{radar}}}\sum_{s \leq S }
  \frac{1}{s}
|\mathcal{RD}_\text{prediction} - \mathcal{RD}_C|.
\end{equation}
As convexity is required for minimization via gradient descent, the sign of the difference is omitted by introducing the value function.

\subsection{Results}\label{se:rcsResults}
The \text{SNR}-\text{NN} neural network is optimized on our dataset as described before. Qualitative results can be found in Fig. \ref{fig:rcs}. By closer inspection, artefacts present in the aspect angle maps (mostly in regions depth was mostly sparse from lidar scanner) can be relocated in the estimated SNR maps $\mathcal{RD}_\text{prediction}$. We conclude, that the NN learned dependencies between the aspect angle feature map from reference sensors and the radar received power. A significant portion in the $\mathcal{RD}_C$ images is suppressed (dark blue area), as it is not covered by the radars FoV, whilst the NN is designed to generalize the same regions in $\mathcal{RD}_\text{prediction}$.

%This happens, because the trained network learned dependencies between the aspect angle feature map from reference sensors and the radar received power, which motivates us in the main part of this work, to use aspect angle for target detection training.

\begin{figure}[tb]
\centering
    \scalebox{1}{\input{Results/RCS/evaluation5.tex}}
    \caption{\textbf{Qualitative results of SNR prediction on test data}. Each yellow block corresponds to one sample frame. In the block, the upper row visualizes the feature maps for the neural network (rgb image, depth image, semantic mask, aspect angle image). The lower rows show the predicted SNR by the neural network and the warped SNR (only pixels from radar FoV) from radar spectra against which the neural network is trained.}
    \label{fig:rcs}
\end{figure}

\section{Conclusions}
In this material, the automatic labeling framework has also been tested in the applications of target detection, semantic segmentation and SNR estimation from camera. In all applications the trained NNs were able to produce reasonable predictions, even though label noise can be attributed to imperfection such as warping errors and erroneous aspect-angle estimation.
